# Supplementary material for: Reinforcement Learning for Slate-based Recommender Systems: A Tractable Decomposition and Practical Methodology
Source: arXiv:1905.12767 source file (2019-05-31)
Supplement: Supplementary file 1 [file appendix.tex]

\section{Appendix: User Simulation Environment}
\label{sec:simulator}

We provide a full description of the simulation models used to test \SlateQ{}, including
all parameters used in our experiments. The simulation model is intentionally 
simplified and stylized to
allow systematic experimentation with different aspects of the \SlateQ{} model.

\vspace*{1mm}
\noindent
\textbf{Document and Topic Model:\ }
We assume a set of documents $D$ representing content to be recommended
and set of topics (or user interests)
$T$ that these documents cover. Each document is characterized by a
\emph{mixture of topics} and some inherent \emph{quality}. While
the model can generally allow documents to have different lengths, we
assume each has constant length $\ell$ (e.g., length of a video, music track or
news article).
We use no other features, with these components characterizing the most
important factors influencing long-term user engagement.

With respect to topics, we can treat $d\in D$ as a topic vector
$\bfd \in [0,1]^{|T|}$. For simplicity, in our experiments, each $d$ has only a
single topic, so we use a one-hot encoding with $\bfd = \bfe_i$ for some $i\leq |T|$,
We write $T(d)$ to denote $d$'s topic. $T(d)$ is observable to the RL
algorithm. We assume some content distribution $P_D$ from which
documents are drawn.

Documents also have an \emph{inherent quality}
% $L_d\in [-1,1]$, drawn
$L_d$, drawn
randomly from the normal distribution $\calN(\mu_{T(d)},\sigma^2)$,
% (and truncated),
where $\mu_t$ is a topic-specific
mean quality for any $t\in T$ (all topics have the same variance in quality). Quality is
unobservable to the RL model.\footnote{In principle, quality can be estimated over time from
user responses (see below) and may also be user-dependent. We do not consider these in
our stylized experiments to focus on the RL methods' ability on learning average 
quality at the topic level.}

In our experiments, we use $T=20$ topics; the number of documents $|D|$ is immaterial (see System
Dynamics below). Of these, $14$ topics are are ``low'' quality, with their mean quality $\mu_t \in [-3,0]$:
the 14 topics have means evenly distributed across this interval. The remaining $6$ topics are
``high'' quality, with $\mu_t \in [0,3]$ and the 6 means distributed evenly across this interval.

\vspace*{1mm}
\noindent
\textbf{User Interest and Satisfaction Models:\ }
Users $u\in U$ are characterized by their interests in topics, ranging from $-1$ (completely
uninterested) to $1$ (full interested), with each $u$ represented by
an interest vector $\bfu\in [-1,1]^{|T|}$.
User $u$'s \emph{interest in document} $d$ is given by the dot product $I(u,d) = \bfu\bfd$. We assume
some prior distribution over user interests $P_U$. A user's interest vector is, however, influenced
by their document consumption (see below). To focus on how well our RL methods handle
learning to influence user interests and the quality of consumption, we treat a
user's interest vector $\bfu$ as fully observable.\footnote{In general, user interests are
latent, and a partially observable/belief state model is more appropriate. Again, we make
this simplifying assumption to focus on the RL methods' ability
learning average quality at the topic level.}
A user's \emph{satisfaction} $S(u,d)$ with a selected/consumed
$d$ is a function $f(I(u,d),L_d)$ of $u$'s interest and $d$'s quality.
We assume a simple convex combination $S(u,d) = (1-\alpha) I(u,d) + \alpha L_d$.

In our experiments, a new user $u$'s prior interest $\bfu$ is sampled uniformly from
$\bfu\in [-1,1]^{|T|}$; specifically, there is no prior correlation across topics.
We use an extreme value of $\alpha = 1.0$ so that a user's satisfaction with a consumed document
is fully dictated by document quality; this leaves user interest to drive the selection of
the document from the slate.\footnote{Experiments with $\alpha < 1$ exhibit qualitatively similar results.}

\vspace*{1mm}
\noindent
\textbf{User Choice Model:\ }
When presented with a slate of $k$ documents, a \emph{user choice} model impacts which item
(if any) from the slate is consumed by the user. We assume that a user \emph{can observe} any
recommended document's topic prior to selection/consumption, but \emph{cannot observe} its quality
before consumption. However, the user will observe the true document quality \emph{after}
consuming it.

Our primary choice model (and the one
upon which $\SlateQ{}$ is based), is a simple \emph{multinomial proportional model},
which is an unexponentiated analog of a multinomial logit model. User $u$'s interest
in $d$, $I(u,d) = \bfu\bfd$, defines it's ``item-level pCTR.'' We then 
normalize to determine the odds of selection from a slate $A$:
$$\pctr_M(d_i, A) = I(u,d_i)/\sum_{d_j \in A} I(u,d_j).$$
To handle the possibility of no click,
we use a fictitious $k+1$st \emph{null} item in each slate, which (for simplicity) has
constant utility for each $u$.

We consider a second-choice model, an \emph{exponential cascade model}, that
accounts for item position on a slate. This choice model assumes ``attention''
is given to one item at a time, with exponentially decreasing attention given to items as
a user moves down the slate. The probability that the document in position $j$
is inspected is $\beta_0\beta^j$, where $\beta_0$ is a ``base inspection''
probability and $\beta$ is the inspection decay. If an item is given attention, then it is
selected with a ``base choice probability'' $P(u,d)$ (in this case,
identical to the proportional model); if
the item in position $j$ is not examined or selected/consumed, then the user proceeds to the
$j+1$st item. The probability that the item in position $j$ is clicked is:
$$\pctr_C(d_j,A) = \beta_0 \beta^{j}\pctr_M(d_j, A).$$
While the cascade model allows for the possibility of no click,
even without the fictitious null item (due to
inspection odds), we keep the null item to allow the $\pctr_M$ term to remain calibrated.
In our experiments, we use $\beta_0 = 1.0$, $\beta = 0.65$.

% A vector of size C, indicating how much of a certain topic a video contains. Properties can range from 0 to +1. For this experiment, we assume the property is a 1-hot vector activated at its cluster ID. 
% Video Length: An integer representing the length of the video. For simplicity, we assume all videos are the same length (4 time units)
% Quality: A float representing the intrinsic “quality” (i.e. trashiness/nutritiousness) of a video. We assume quality is sampled from a normal distribution with a mean based on the cluster ID, and fixed variance. Quality ~ N (muK, sigma2). Cluster means are biased, with 70% of the clusters falling equally spaced from [-3, 0] (i.e. the trashy clusters) and the remaining 30% are spaced from [0, 3] (good clusters).

\vspace*{1mm}
\noindent
\textbf{User Dynamics:\ }
To model long-term planning, we assume $u$ has an initial (unobservable)
\emph{budget} $B_u$ of time
to engage with content during an extended session.\footnote{Other models that
do not use terminating sessions are possible of course, and could emphasize
amount of engagement per period.} Each $d$ consumed reduces $u$'s budget, with
a session ending once $B_u$ reaches $0$. The budget decreases
by the fixed document length $\ell$ (this can easily vary per item if desired) less a ``bonus'' $b$
that increases with $S(u,d)$; thus, more satisfying items decrease the time remaining in a
session at a lower rate. (Since sessions terminate with probability 1,
discounting is unnecessary.) In our experiments, each user's initial budget is $B_u = 200$ units
of time; each consumed item uses $\ell =4$ units; and if a slate is recommended, but no item is clicked,
$0.5$ units are consumed. We set bonus $b = \frac{0.9}{3.4}\cdot \ell \cdot S(u,d)$.

When $u$ consumes $d$, her interest in topic $T(d)$ is nudged
stochastically, biased slightly toward increasing her interest, but allows some chance
of decreasing her interest. Thus, a recommender faces a short-term/long-term
tradeoff between nudging a user's interests toward topics that tend to have higher quality
at the expense of short-term consumption of user budget. We use the following stylized
model to set the magnitude of the adjustment (how much the interest in topic $T(d)$ changes) and
its polarity (whether it increases or decreases). Let $t=T(d)$ be the topic of the consumed document
$d$ and $I_t$ be $u$'s interest in $t$ prior to consumption of $d$. The (absolute) change $\Delta_t(I_t)$
in $u$'s interest is $\Delta_t(I_t) = (-y |I_t| + y)\cdot -I_t$, where $y\in [0,1]$ sets the fraction
of the distance between the current interest level and the maximum level (1, -1) that the update
move $u$'s interest (so more extreme or ``entrenched'' interests change less than ``neutral''
interests). In our experiments we set $y = 0.3$.
A positive change in interest, $I_t\leftarrow I_t + \Delta_t(I_t)$, occurs with probability
$[I(u,d)+1]/2$, and a negative change, $I_t\leftarrow I_t - \Delta_t(I_t)$, with probability
$[1-I(u,d)]/2$. Thus positive (resp., negative) interests are more likely to be reinforced,
i.e., become more positive (resp., negative), with the odds of such
reinforcement increasing with
the degree of ``entrenchment.''

\vspace*{1mm}
\noindent
\textbf{Recommender System Dynamics:\ }
At each stage of interaction with a user, $m$ \emph{candidate} documents are drawn from $P_D$,
from which a slate of size
$k$ must be selected for recommendation. This reflects the common situation in many large-scale
commercial recommenders in which a variety of mechanisms are used to sub-select a small set of
candidates from a massive corpus, which are then in turn scored using more refined (and computationally
expensive) predictive models
of user engagement. We use $m=10,k=3$ in these synthetic experiments to
allow comparison to a method that enumerates slates; in our live experiments, slates are of variable
size and the number of candidates is on the order of $O(1000)$.

A user selects a document(or possibly no-clicks) according to the specified choice model,
and her budget and interests are updated according to the user dynamics model.

% \vspace*{1mm}
% \noindent
% \textbf{Summary of Observable, Unobservable Properties:\ }
% None of $P_D$, $P_U$, $\mu_t, t\in T$ or $\sigma^2$ are known \emph{a priori} to the RL algorithm.

\section{Appendix: User Simulation}

We train the models in our synthetic experiments as follows: each episode corresponds to the
system interacting with a single user. The user's interest vector $\bfu$ is drawn from $P_u$ and
the system interacts with that user until her time budget $B_u$ is consumed. At that point, another
user is drawn. It is also possible to interleave users (as would arise in a live recommender), but
this rate of learning and final policy/Q-function learned vary negligibly under either
choice.\footnote{In synthetic experiments, we needn't worry about the potential negative
effects on user's engaged during early stages of training.}

We train our policies using $\veps$-greedy training, with $\veps = 0.1$. Evaluation of the
greedy policy induced by the current \SlateQ{} model is done continuously using a random
sample of 50 user-sessions. Training performance curves use an exponentially smoothed average
of all past evaluations (the evaluation $t$ stages ago is discounted by $\zeta^t$ (we use
$\zeta = 0.999$). 

Our primary metric is the expected total user engagement (i.e., session time) of the policy;
but we also consider the average quality of the recommendations consumed by users under different policies. Fig.~\ref{fig:learningcurve2} and Fig.~\ref{fig:learningcurve3} illustrate how the LTV and MYOP policies learn to prefer different quality topics over time.

\begin{figure}[t]
\centering
  \includegraphics[width=0.65\linewidth]{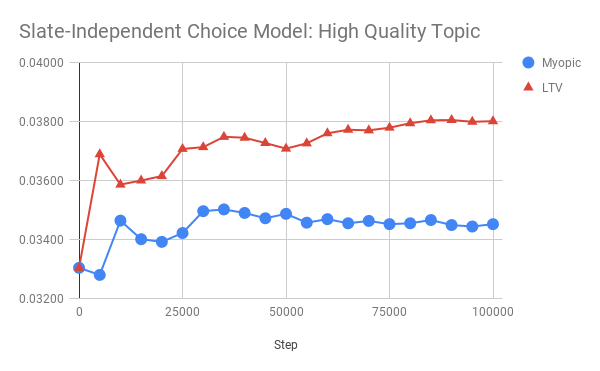}
  \vspace*{-3mm}
  \caption{Learning Curves for High Quality Topic.}
  \vspace*{-3mm}
  \label{fig:learningcurve2}
\end{figure}

\begin{figure}[t]
\centering
  \includegraphics[width=0.65\linewidth]{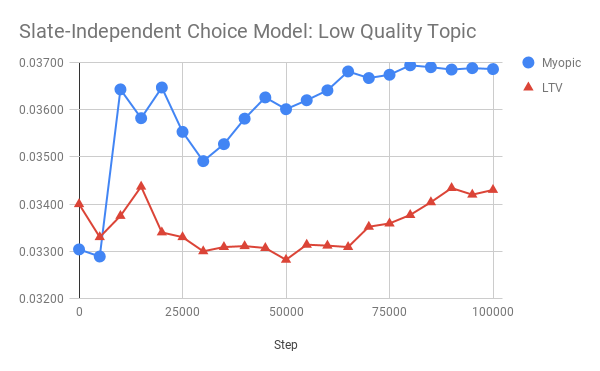}
  \vspace*{-3mm}
  \caption{Learning Curves for Low Quality Topic.}
  \vspace*{-3mm}
  \label{fig:learningcurve3}
\end{figure}

\section{Appendix: A Practical Methodology}
\label{sec:implementation}

The deployment of a recommender using RL or TD methods to optimize
for long-term user engagement presents a number
of challenges in practice. In this section, we identify several of
these and suggest practical techniques to resolve them, including ways in
which to exploit an existing \emph{myopic}, item-level recommender to
facilitate the deployment of a non-myopic system.

Many (myopic) item-level recommenders 
\cite{liu2009letor,covington:recsys16} have the following
components: (i) \emph{Logging} of impressions and user feedback;
(ii) \emph{Training} of some regression model (e.g., DNN)
to predict user responses for user-item pairs, which are then
aggregated by some scoring function; and (iii) \emph{Serving} of
recommendations, ranking items by score (e.g.,
returning the top $k$ items for recommendation).
% \begin{enumerate}
%     \item \emph{Training}: A regression model that predicts a score for each (user, item) pair.
%     \item \emph{Serving}: A ranker that ranks items based on the scores of the regression model and returns the top $K$ items.
%     \item \emph{Logging}: The impressions and users' feedback will be logged as examples and labels, which are then used for training.
% \end{enumerate}
We can exploit such a system to quickly develop a non-myopic
recommender based on Q-values (i.e., predictions of long-term user
engagement) by addressing several key challenges.

\noindent
\textbf{State Space Construction.}\hskip 2mm
A critical part of any RL modeling is the design of the state
space, that is, the development of a set of features that
adequately capture a user's past history to allow prediction of
long-term value (e.g., engagement) in response to a recommendation.
For the underlying process to be an MDP, the feature set should be
(at least approximately) predictive of immediate user response
(e.g., immediate engagement, hence \emph{reward}) and ``self-predictive''
(i.e., summarizes user history in a way that renders the implied dynamics Markovian).

The features of an extant myopic recommender typically satisfy
both of these requirements, meaning that an RL or TD model can be
built using the same logged data (organized into trajectories)
and the same featurization. The engineering, experimentation and experience
that goes into developing state-of-the-art recommenders means that
they generally capture (almost) all aspects of history required
to predict immediate user responses (e.g., pCTR, listening time,
 other engagement metrics); i.e., they form a sufficient statistic. 
In addition, the core input features
(e.g., static user properties, summary statistics
of past behavior and responses) are often self-predictive
(i.e., no further history could significantly improve next state
prediction).\footnote{This fact can often be verified by inspection
and semantic interpretation of the (input) features.}
Thus, using the existing state definition
provides a natural, practical way to construct TD or RL models.
We provide experimental evidence below to support this assertion.

\noindent
\textbf{Generalization across Users.}\hskip 2mm
While each user should be viewed as a separate environment
or MDP, it is critical to allow for generalization across users (a hallmark
of almost any recommender system)---in this case, we need to generalize
the (implicit) MDP dynamics across users. The state representation afforded
by an extant myopic recommender is already intended to do just this.

\noindent
\textbf{User Response Modeling.}\hskip 2mm
As noted above,
% in Sec.~\ref{sec:setup},
\SlateQ{} can exploit a pCTR model to capture
user choice behavior. Since myopic recommenders often predict exactly such
responses, we can use these models directly. Furthermore, by using the
same state features (see above), it is straightforward to build a
multi-task model \cite{zhang2017asurvey} that incorporates our long-term engagement
prediction with other user response predictions.

\noindent
\textbf{Logging, Training and Serving Infrastructure.}\hskip 2mm
The training of long-term values $Q^\pi(s,i)$ requires logging of user
data, and live serving of recommendations based on these LTV scores. The model architecture we detail below
exploits the same logging, (supervised) training and serving infrastructure
as used by the myopic recommender.

% \noindent
% \textbf{Reward Function Design.}\hskip 2mm \textbf{TODO: Maybe add a comment
% or two on this?}

Fig.~\ref{fig:system_overview} illustrates the structure of our LTV-based recommender.  In myopic recommenders, the regression model predicts
immediate user response (e.g., clicks, engagement), while in
our non-myopic recommender, label generation provides LTV labels,
allowing the regressor to model $\qbar^\pi(s,i)$.
\begin{figure}[t]
\centering
  \includegraphics[width=0.45\linewidth]{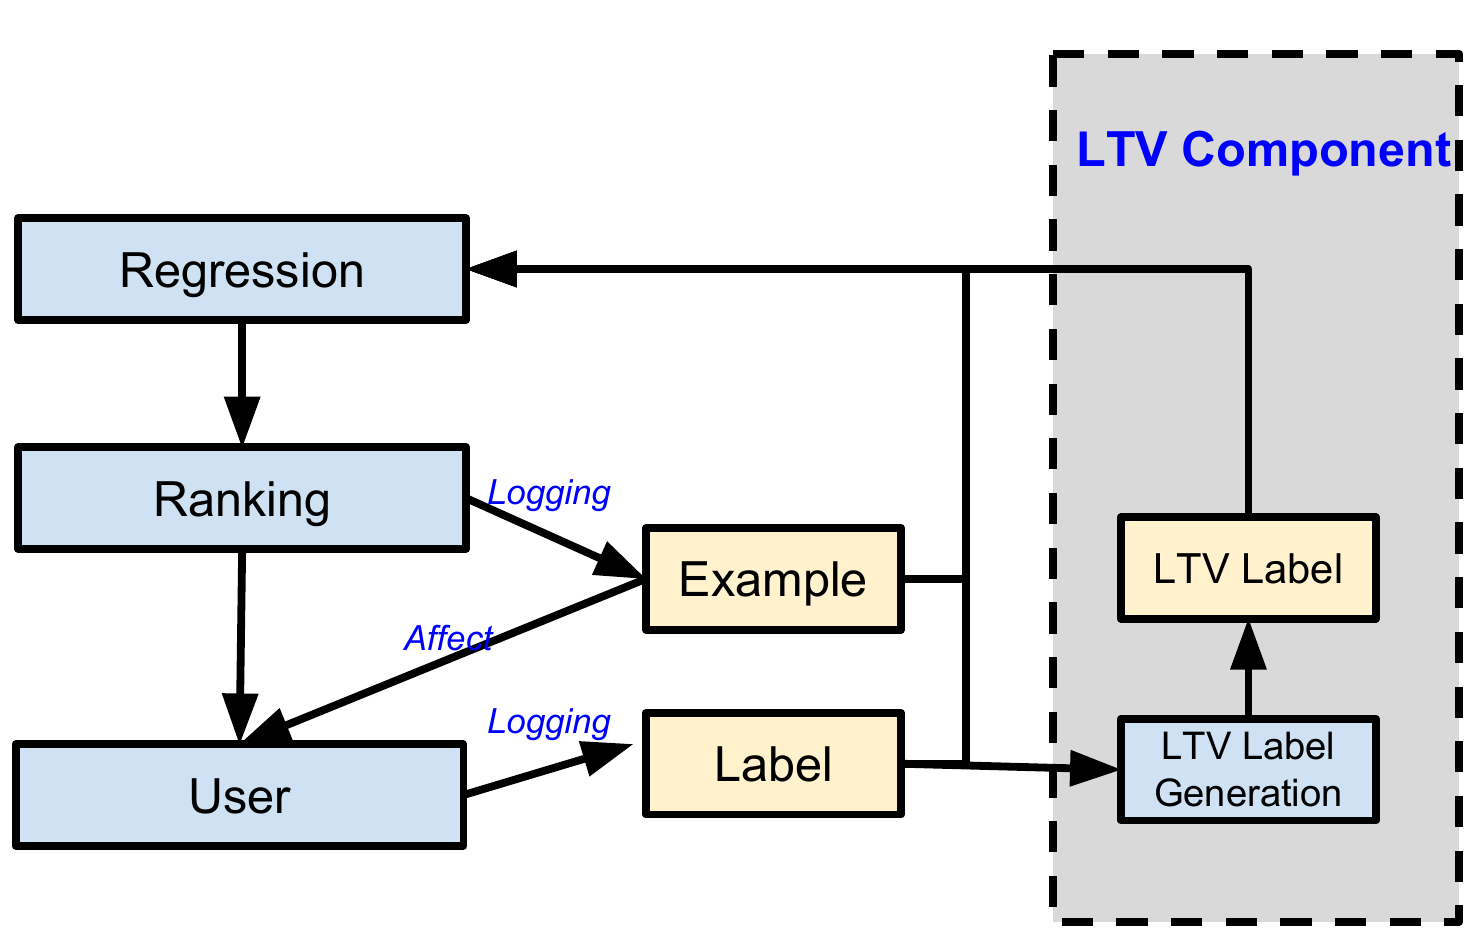}
    \vspace*{-2mm}
  \caption{Schematic View of a Non-myopic Recommender Training System}
  \label{fig:system_overview}
    \vspace*{-3mm}
\end{figure}
Models are trained periodically and pushed to the server
(e.g., \cite{baylor2017tfx}). The ranker uses the latest model
to recommend items and logs user feedback,
which is used to train new models.
Using LTV labels, iterative model training and pushing
can be viewed as a form of \emph{generalized policy
iteration}~\cite{sutton:rlbook}. Each trained DNN represents the value of the policy that generated the prior batch of
training data: thus training is effectively
\emph{policy evaluation}.
The ranker acts greedily with respect to this value function, thus performing
\emph{policy improvement}.

% (For information only): see go/sl-rl-unify for more background of the generalized policy iteration item.

LTV label generation is similar to DQN training
\cite{mnih2015}: a main network learns the LTV of individual items, $\qbar^\pi(s,i)$,
(easily extended from the existing myopic DNN); for 
stability, LTV (bootstrapped) labels are generated using a separate 
label network.  We periodically copy the weights of the main network to 
the label network and use the (fixed) label network $\qbar_{label}(s, i)$ to compute LTV labels 
between copies.  LTV labels are generated as follows (see Eq.$12$):
\begin{small}
\begin{equation}
\qbar(s, i)=r(s,i)+ \gamma \sum_{j\in A'} \pctr(s',j,A')\qbar_{label}(s',j)
\label{eq:ltv_label_compute}
\end{equation}
\end{small}
% where $r(s,a)$ is the myopic label, $Q_{label}(\cdot,\cdot)$ is the output of
% the label network, and $p(a|s)=pctr(s, a)/\sum_{a'\in A} pctr(s, a')$
% is the normalized pCTR.  To get 
We use a multi-task network \cite{zhang2017asurvey}
to allow $\pctr(s, i)$ prediction along with
(conditional-on-click) Q-values $\qbar(s,i)$.
% multi-task feedforward neural network \cite{zhang2017asurvey}.  One
% output of the network predicts the long-term value of the video, the
% other predicts the pCTR.
% Our complete training algorithm is described in
% supplementary Appendix~\ref{sec:algorithm}.

\section{Appendix: Live Experiment Training and Further Results}
\label{sec:algorithm}

The large-scale live experiment was run using the \SlateQ{} approach discussed in the main
body of the paper. Here we specify a few additional details and experimental results.

\vspace*{1mm}
\noindent
\textbf{Model Architecture:\ }
\begin{figure}
\centering
   \includegraphics[width=0.7\linewidth]{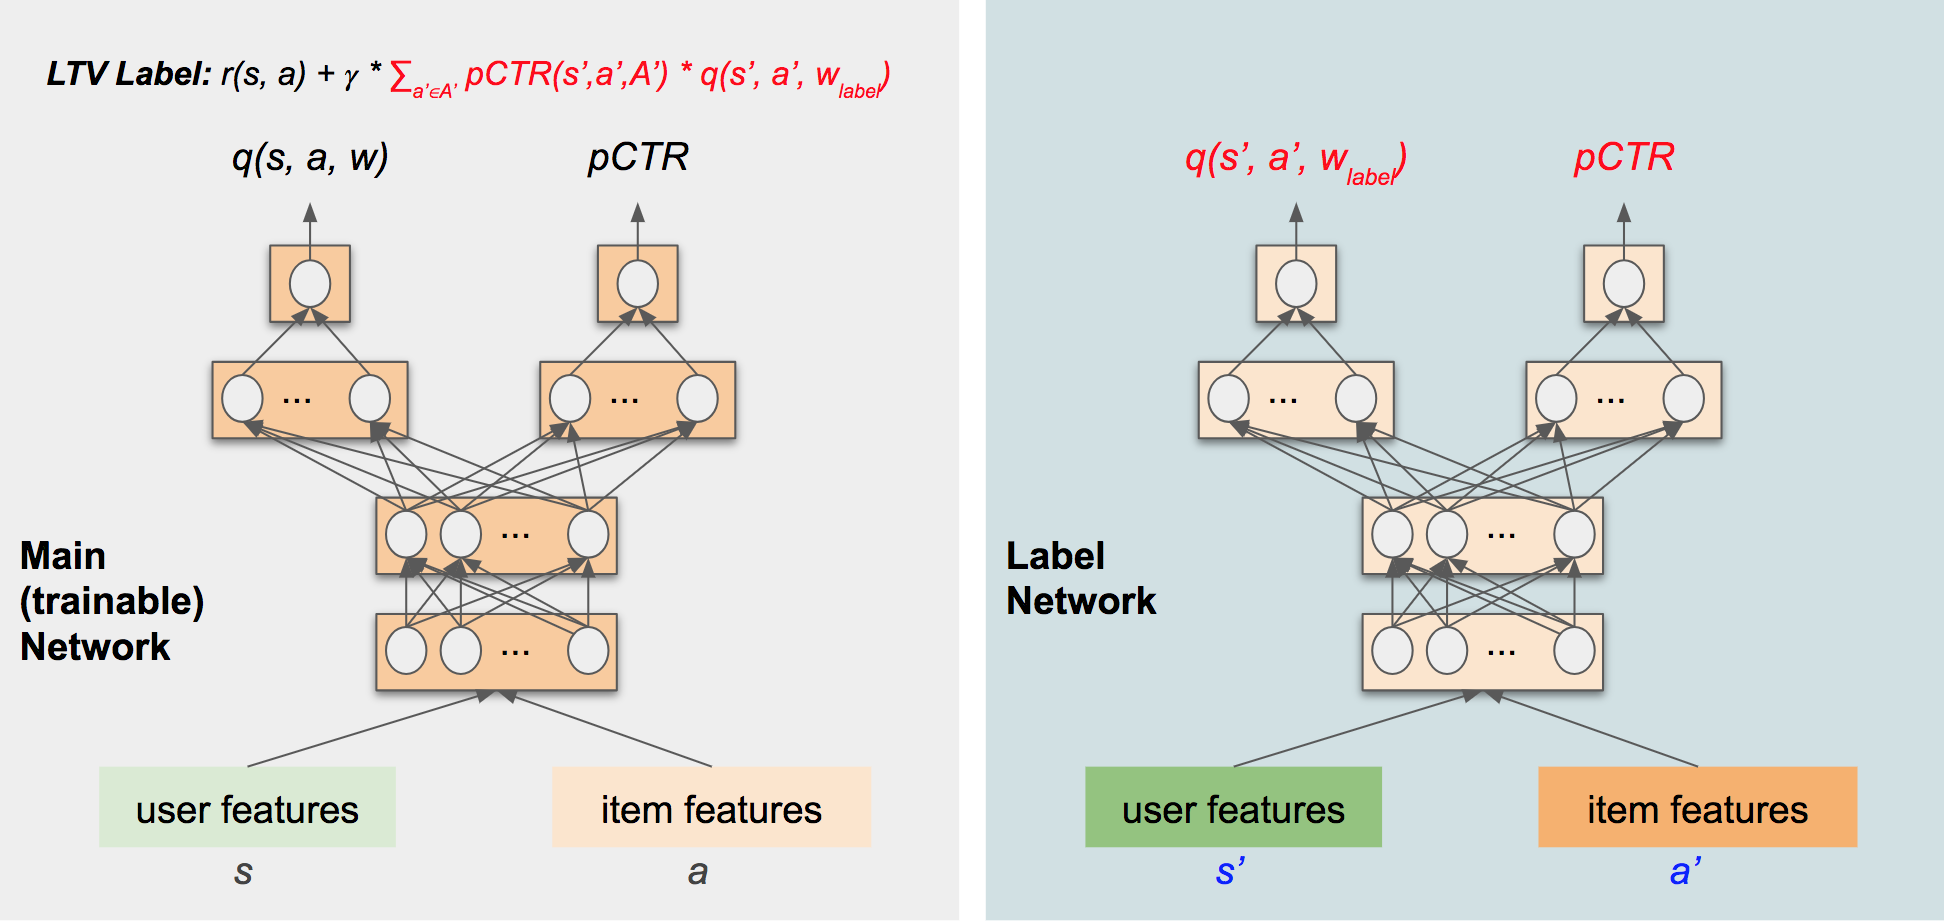}
     \vspace*{-2mm}
   \caption{Model Architecture}
   \label{fig:network-architecture}
     \vspace*{-3mm}
\end{figure}

We extend the recommender's current ranking model to a multi-task
feedforward neural network \cite{zhang2017asurvey} that learns 
$\qbar(s, i)$, the predicted long-term engagement of item $i$
conditional on it being clicked by a user in state $s$, as well as
$\pctr(s, i)$.
% or predicted click-through rate on given video $a$ in given context $s$.  
Training is over pairs of consecutive start page
visits, and LTV labels are computed using Eq.~\ref{eq:ltv_label_compute} as
depicted in Fig.~\ref{fig:network-architecture}.

We use a feed forward, multitask/head DNN network with 4 hidden layers of sizes 2048, 1024, 512, 256;
and used ReLU activation functions on each of the hidden layers. Apart from the LTV/Q-value head, other heads include pCTR, and other user responses. To validate our methodology, the DNN structure and all input features are identical to the production model which optimizes for short-term (myopic) immediate reward. The state is defined by user features (e.g., user’s past history, behavior and responses, plus static user attributes). This also makes the comparison with the baseline fair.

\vspace*{1mm}
\noindent
\textbf{Training Algorithm:\ }
The full training algorithm used in our live experiment is
shown in Algorithm~\ref{algorithm:training}.

\begin{small}
\begin{algorithm}
  \caption{Our Algorithm}
  \begin{algorithmic}[1]
  \label{algorithm:training}
    \STATE \textbf{Parameters:} $T$: the number of iterations. $M$: the interval to update label network. $\gamma$:  discount rate. $\theta_{main}$: the parameter for the main neural network $\qbar_{main}$ that predicts items' long-term value. $\theta_{label}$: the parameter for the label neural network $\qbar_{label}$. $\theta_{pctr}$: the parameter for the neural network that predicts items' pCTR.
    \STATE \textbf{Input:} $D_{training}=(s,A,C,L_{myopic}, s', A')$: the training data set.
    \begin{itemize}
     \item $s$: current state features
     \item $A=(a_1,... ,a_k)$: recommended slate of items in current state; $a_{i}$ denotes item features
     \item $C=(c_1,...,c_k)$: $c_{i}$ denotes whether item $a_{i}$ is clicked
     \item $L_{myopic}=(l^{1}_{myopic},...,l^{k}_{myopic})$: myopic (immediate) labels
     \item $s'$: next state features
     \item $A'=(a_1',... ,a_k')$: recommended slate of items in next state.
    \end{itemize}
    \STATE \textbf{Output:} Trained Q-network $\qbar_{main}$ that predicts items' long-term value.
    
    \STATE \textbf{Initialization} $\theta_{label}=0$, $\theta_{main}$ randomly, $\theta_{pctr}$   randomly
    \FOR{$i = 1 \dots T$}
      \IF{$i \bmod  M = 0$}
        \STATE$\theta_{label} \leftarrow \theta_{main}$
      \ENDIF
      
      \FOR{each example $(s,A,C,L_{myopic}, s', A') \in D_{training}$}
        \FOR{each item $a_i \in A$}
          \STATE update $\theta_{pctr}$ using click label $c_i$
          \IF{$a_i$ is clicked}
            \STATE compute probability    $\pctr(s', a_i', A')\leftarrow \pctr(s', a_i')/\sum_{a_i'\in A}pctr(s', a_i')$
            \STATE compute LTV label: $l^i_{ltv}\leftarrow l^i_{myopic} +\sum_{a_i'\in A'}\pctr(s', a_i', A') \qbar_{label}(s', a_i')$ 
            \STATE update $\theta_{main}$ using LTV label $l^i_{ltv}$
          \ENDIF
        \ENDFOR
      \ENDFOR
    \ENDFOR
  \end{algorithmic}
\end{algorithm}
\end{small}

Fig.~\ref{fig:calibration_plot} shows the calibration plot for
our model: we group all clicked impressions into $100$ quantiles
based on predicted LTV score; for each quantile-bucket,
we compute the average predicted LTV score and (i) (left plot)
average observed immediate engagement (or reward) and (ii)
average observed long-term engagement (or the ``TD(1)-label'').
The strong calibration between predicted and observed LTV label validates
the hypothesis that the features of the myopic recommender provide a
reasonable state representation for Q-value/LTV prediction using SARSA.

% The data source of this figure is stored at /cns/vk-d/home/jingconanwang/ttl=720d/qydra/calibration_20180420_20180501_23735973/data-00000-of-00001
% Please see this colab for how to generate the calibration plot: https://colab.corp.google.com/drive/1JTZo31TEGPeBLfljoTlHVKIb-QksSTzf#scrollTo=wdjqYVW_9gMm

\begin{figure}
\centering
   \includegraphics[width=0.75\linewidth]{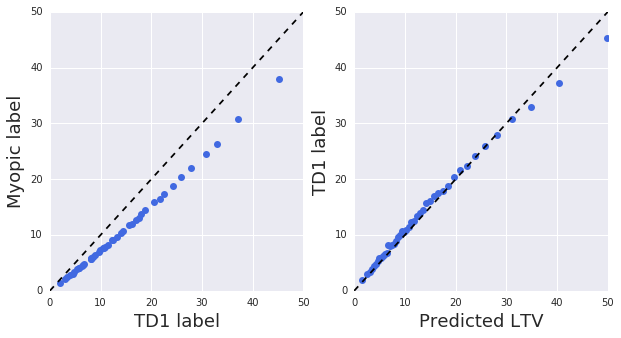}
     \vspace*{-3mm}
   \caption{Calibration plots: relationship between myopic and TD(1) labels (left) and TD(1) labels and LTV predictions (right).}
   \label{fig:calibration_plot}
     \vspace*{-3mm}
\end{figure}
